# Supplementary material for: NUMAscope: Capturing and Visualizing Hardware Metrics on Large ccNUMA Systems
Source: arXiv:2111.11836 source file (2021-11-23)
Supplement: Supplementary file 1 [file appendix.tex]

\section{NumaConnect2 events}
\label{appendix:events}

The list of events in the Numascale second generation interconnect is:
\begin{itemize}
\item cycles
\item cycles at least half of the available RMPE contexts were in use
\item cycles the RMPE had free contexts for SIU accesses
\item cycles the RMPE had free contexts for PIU accesses
\item requests from PIU to RMPE
\item valid cycles acked for requests from PIU to RMPE
\item wait cycles for requests from from PIU to RMPE
\item responses from PIU to RMPE
\item valid cycles acked for responses from PIU to RMPE
\item wait cycles for responses from from PIU to RMPE
\item requests from SIU to RMPE
\item valid cycles acked for requests from SIU to RMPE
\item wait cycles for requests from from SIU to RMPE
\item responses from SIU to RMPE
\item valid cycles acked for responses from SIU to RMPE
\item wait cycles for responses from from SIU to RMPE
\item cycles at least half of the available LMPE contexts were in use
\item cycles the LMPE had free contexts for SIU accesses
\item cycles the LMPE had free contexts for PIU accesses
\item requests from PIU to LMPE
\item wait cycles for requests from from PIU to LMPE
\item responses from PIU to LMPE
\item valid cycles acked for responses from PIU to LMPE
\item wait cycles for responses from from PIU to LMPE
\item requests from SIU to LMPE
\item valid cycles acked for requests from SIU to LMPE
\item wait cycles for requests from from SIU to LMPE
\item responses from SIU to LMPE
\item valid cycles acked for responses from SIU to LMPE
\item wait cycles for responses from from SIU to LMPE
\item VicBlk and VicBlkClean commands received
\item RdBlk and RdBlkS commands received
\item RdBlkMod commands received
\item ChangeToDirty commands received
\item RdSized commands received
\item WrSized commands received
\item directed Probe commands received
\item broadcast Probe commands received
\item Broadcast commands received
\item RdResponse commands received
\item ProbeResponse commands received
\item data packets with full cachelines of data received
\item data packets with less than a full cache line received
\item VicBlk and VicBlkClean commands sent
\item RdBlk and RdBlkS commands sent
\item RdBlkMod commands sent
\item ChangeToDirty commands sent
\item RdSized commands sent
\item WrSized commands sent
\item broadcast Probe commands sent
\item broadcast commands sent
\item RdResponse commands sent
\item ProbeResponse commands sent
\item data packets with full cachelines of data sent
\item data packets with less than a full cache line sent
\item nCache read hits on RMPE
\item nCache store hits on RMPE
\item nCache store misses on RMPE
\item nCache roll outs on RMPE
\item nCache invalidates on RMPE
\item cycles with at least one free Hreq context in PIU
\item cycles with at least one free Pprb context in PIU
\item cycles with at least one free Hprb context in PIU
\item cycles with at least one free Preq context in PIU
\item accesses to C/Mtag cache 0..3
\item write hit accesses to C/Mtag cache 0..3
\item read hit accesses to C/Mtag cache 0..3
\item write accesses with writebacks to C/Mtag cache 0..3
\item read accesses with writebacks to C/Mtag cache 0..3
\item write miss accesses to C/Mtag cache 0..3
\item read miss accesses to C/Mtag cache 0..3
\end{itemize}

There are 56 discrete hardware counters for the last seven in the list, covering the cache-tag and main-memory-tag functional units, each of which are 4-way striped by physical address.

%%% Local Variables:
%%% mode: latex
%%% TeX-master: "paper"
%%% End:
